# Supplementary material for: Understanding and Evaluating Hallucinations in 3D Visual Language Models
Source: arXiv:2502.15888 source file (2025-02-18)
Supplement: Supplementary file 1 [file 6.appendix.tex]

% \newpage
\section{Appendix}
